# Supplementary material for: Dialing back time on Timepix3: A study on the timing performance of Timepix3
Source: arXiv:2201.09275 source file (2022-01-23)
Supplement: Supplementary file 3 [file AppendixFiguresList.tex]

%\listoffigures
